# Supplementary material for: Measuring and Predicting Where and When Pathologists Focus their Visual Attention while Grading Whole Slide Images of Cancer
Source: arXiv:2508.01668 source file (2025-08-03)
Supplement: Supplementary file 1 [file supplement.pdf]

# Supplementary: Measuring and Predicting Where and When Pathologists Focus their Visual Attention while Grading Whole Slide Images of Cancer

Souradeep Chakraborty<sup>a</sup>, Ruoyu Xue<sup>a</sup>, Rajarsi Gupta<sup>b</sup>, Oksana Yaskiv<sup>d</sup>,  
Constantin Friedman<sup>d</sup>, Natallia Sheuka<sup>d</sup>, Dana Perez<sup>d</sup>, Paul Friedman<sup>d</sup>,  
Won-Tak Choi<sup>f</sup>, Waqas Mahmud<sup>b</sup>, Beatrice Knudsen<sup>e</sup>, Gregory Zelinsky<sup>c</sup>,  
Joel Saltz<sup>b</sup>, Dimitris Samaras<sup>a</sup>

<sup>a</sup>*Department of Computer Science, Stony Brook University, Stony Brook, 11794, NY, USA*

<sup>b</sup>*Department of Biomedical Informatics, Stony Brook University, Stony Brook, 11794, NY, USA*

<sup>c</sup>*Department of Psychology, Stony Brook University, Stony Brook, 11794, NY, USA*

<sup>d</sup>*Department of Pathology and Laboratory Medicine, Northwell Health Laboratories, Greenvale, 11548, NY, USA*

<sup>e</sup>*Department of Pathology, University of Utah School of Medicine, Utah, 84112, NY, USA*

<sup>f</sup>*Department of Pathology, University of California San Francisco, San Francisco, 94143, CA, USA*

---

## 1. Token Similarity of Scanpaths Metric (TokSimScan)

For a given WSI at inference, the *TokSimScan* metric averages the cosine similarity score between the feature tokens computed for each viewport in the predicted scanpath and the tokens computed for each viewport in the pathologist-derived scanpaths (ground truth data), aggregated across all pathologists who viewed the WSI. We formulate the *TokSimScan* metric as follows:

$$\text{TokSimScan} = \frac{1}{N} \sum_{i=1}^N \frac{1}{K} \sum_{k=1}^K \frac{\mathbf{F}_i^{\text{pred}} \cdot \mathbf{F}_i^{(k)}}{\|\mathbf{F}_i^{\text{pred}}\|_2 \|\mathbf{F}_i^{(k)}\|_2}, \quad (1)$$

where  $N$  is the number of viewports in the predicted scanpath,  $K$  is the number of pathologists who viewed the WSI,  $\mathbf{F}_i^{\text{pred}}$  is the feature token vector computed for the  $i$ -th viewport in the predicted scanpath,  $\mathbf{F}_i^{(k)}$  is the feature

token vector computed for the  $i$ -th viewport in the scanpath of the  $k$ -th pathologist.  $\|\cdot\|_2$  denotes the  $L_2$  norm of a vector.

Our motivation for introducing *TokSimScan* is twofold:

- 1) **Scalability:** Unlike SSS, which is limited to 13 WSIs with tumor segmentation annotations, the *TokSimScan* metric can scale across the entire dataset using cross-validation. This flexibility makes it applicable even in cases where semantic annotations are sparse, thereby improving scalability.
- 2) **Enhanced Semantics:** Gleason grades used in SSS do not fully capture the semantic factors influencing a pathologist’s attention. By contrast, feature tokens from our PAT-Heatmap sub-network, trained on pathologists’ attention heatmaps, encode richer semantic information, offering a more comprehensive understanding of attention dynamics.

## 2. Implementation details

For attention heatmap prediction (stage 1), we evaluated two different feature extractors: 1) the ViT-S model (embedding size  $D = 384$ ) trained using DINO, and 2) the (Kang et al., 2023) model pretrained on histopathology data, for extracting WSI patch features (frozen while training). Kang et al. pretrained both ResNet50 and ViT/S architectures; we chose the ViT-based features over CNN-based ResNet50 features due to their more memory- and compute-efficient representation (one token per patch), which aligns better with our transformer-based pipeline. Using CNN features would significantly increase computational cost (by at least 50X), rendering them impractical for our setup. For predicting heatmap, we input grids of variable sizes to our network for different magnifications -  $10 \times 10$  for 2X,  $20 \times 20$  for 4X,  $50 \times 50$  for 10X and  $60 \times 60$  for 20X. Our transformer encoder contains  $n_l = 12$  layers with  $n_h = 8$  attention heads.

For attention scanpath simplification task, we empirically set the scanpath simplification thresholds as follows: angle threshold  $Th_A = 40^\circ$ , temporal duration threshold  $Th_T = 2$  seconds, and dispersion threshold  $Th_D = 12$  units for coordinates in a spatial resolution of  $(80, 128)$ .

For attention scanpath prediction, we evaluated the encoded feature representations of 1) the ViT-S model (embedding size  $D = 384$ ) and 2) the *Kang* model, derived from the attention heatmap prediction sub-network PAT-H. We set the resolution of the low-dimensional 2X features to  $10 \times 16$  and that of the high-dimensional 10X features to  $80 \times 120$  for computational

efficiency during training and inference. Consequently, the size of the predicted heatmap is also  $80 \times 120$ . The MLP in the fixation prediction module has two linear layers with 512 hidden dimensions and a ReLU activation function. The MLP in the magnification prediction module has two linear layers with 64 and 32 hidden dimensions and a ReLU activation function. The maximum trajectory length of our condensed scanpaths is 150.  $\lambda_{Mag}$ , the parameter for the magnification classification loss is empirically set to 1, following (Yang et al., 2024). For both tasks, we used the AdamW optimizer with batch size = 8, learning rate =  $10^{-4}$ , and weight decay =  $10^{-4}$  for training the corresponding sub-networks. At inference time, the length of the predicted scanpath  $S$  was capped to  $len(S) = 60$ , which is the average length of scanpaths in our dataset.

### 3. Evaluation of attention heatmap prediction

**Metrics.** We quantitatively evaluate model performance using three metrics (Bylinskii et al., 2018): Cross Correlation (CC), Normalized Scanpath Saliency (NSS), and KL-Divergence (KLD). Cross Correlation (CC) score quantifies the spatial similarity between two continuous-valued maps, such as a predicted attention heatmap and a ground truth fixation-density map. CC is computed as the Pearson correlation coefficient between the two maps, measuring how well the predicted intensities align with the observed ones. Higher CC values indicate better alignment. Normalized Scanpath Saliency (NSS) evaluates how well the predicted attention heatmap aligns with the actual fixation locations. It normalizes the predicted map by its mean and standard deviation and then calculates the average saliency values at the ground truth fixation points. Higher NSS scores indicate better fixation alignment. KL-Divergence (KLD) measures the dissimilarity between the predicted and ground truth probability distributions of attention. It quantifies how much information is lost when the predicted distribution is used to approximate the ground truth. Lower KLD values signify closer agreement between the two distributions.

**Baselines.** We compare the performance of our stage 1 sub-network PAT-H to four baseline models. Two are frozen feature extractor baselines, “Frozen ResNet50 + Linear Probing” and “Frozen DINO + Linear Probing”. Both use pretrained backbones (ResNet50 and DINO, respectively) with a linear probing layer as the decoder for heatmap prediction. This decoder is a  $1 \times 1$

convolutional layer that reduces the channel dimension from  $D$  (number of feature maps in the backbone) to 1, effectively projecting the feature map into a single-channel spatial map. We also used as baselines the ProstAttNet (Chakraborty et al., 2022b) and PathAttFormer (Chakraborty et al., 2022a) models, which are two more recent architectures specifically designed for predicting the attention of pathologists, with the latter leveraging positional attention mechanisms.

**Results.** In Table 1, we compare the 5-fold cross validation performance of the different baseline models with our models on 25 test H&E WSIs at different magnification levels. Our models trained using the DINO and DINO-v2 feature descriptors outperform the baseline models by a significant margin at each magnification by all metrics.

In Table 2, we compare the attention prediction performance between our PAT-Heatmap model trained on specialist data and our model trained on non-specialist (residents and general pathologists) data. We test these models on 17 H&E WSIs (with tumor annotations from a GU specialist) at different magnifications. While in Table 1 we used pathologist-derived attention heatmaps as the ground truth for evaluating the spatial overlap between the predicted attention heatmaps and the pathologist-derived attention data (heatmaps and viewport fixations), in Table 2 we used binary tumor segmentation maps as the ground truth for measuring the spatial overlap between the predicted attention heatmaps and the tumor segmentation maps. We find that our model trained on specialists’ data performs better than our model trained on non-specialist data on the 4X, 10X and 20X magnifications (the most commonly used for Gleason grading). These results suggest that non-specialist pathologists might benefit from training on the attention behavior of specialists.

In Figure 1, we qualitatively compare the attention heatmaps predicted by our model using DINO (Caron et al., 2021) and DINO-v2 (Oquab et al., 2023) features as input with three baseline models: (1) frozen Resnet50 encoded features + linear probing using a  $2048 \times 1$  convolutional layer as a decoder, (2) frozen DINO encoded features + linear probing using a  $384 \times 1$  convolutional layer as a decoder, (3) ProstAttNet (Chakraborty et al., 2022b) on a test WSI from our dataset. We see that our PAT-Heatmap sub-network produces more accurate attention heatmaps compared to the baselines.

| Model                                   | $CC_{Attn}$                         | $NSS_{Attn}$                        | $KLD_{Attn}$                        |
|-----------------------------------------|-------------------------------------|-------------------------------------|-------------------------------------|
| Frozen ResNet50+Dec.                    | $0.498 \pm 0.214$                   | $0.748 \pm 0.307$                   | $0.383 \pm 0.023$                   |
| Frozen DINO+Dec.                        | $0.486 \pm 0.192$                   | $0.705 \pm 0.275$                   | $0.397 \pm 0.026$                   |
| ProstAttNet (Chakraborty et al., 2022b) | $0.409 \pm 0.159$                   | $0.644 \pm 0.230$                   | $1.633 \pm 0.600$                   |
| PAT-H (w/ DINO)                         | $0.560 \pm 0.199$                   | $0.836 \pm 0.290$                   | $0.362 \pm 0.070$                   |
| PAT-H (w/DINO-v2)                       | $0.551 \pm 0.149$                   | $0.829 \pm 0.202$                   | $0.348 \pm 0.022$                   |
| PAT-H (w/Kang)                          | <b><math>0.799 \pm 0.019</math></b> | <b><math>1.383 \pm 0.138</math></b> | <b><math>0.227 \pm 0.031</math></b> |

(a) 2X

| Model                                   | $CC_{Attn}$                         | $NSS_{Attn}$                        | $KLD_{Attn}$                        |
|-----------------------------------------|-------------------------------------|-------------------------------------|-------------------------------------|
| Frozen ResNet50+Dec.                    | $0.636 \pm 0.067$                   | $1.106 \pm 0.190$                   | $0.512 \pm 0.151$                   |
| Frozen DINO+Dec.                        | $0.595 \pm 0.067$                   | $1.014 \pm 0.207$                   | $0.539 \pm 0.141$                   |
| ProstAttNet (Chakraborty et al., 2022b) | $0.571 \pm 0.052$                   | $0.972 \pm 0.114$                   | $1.148 \pm 0.249$                   |
| PAT-H (w/ DINO)                         | $0.668 \pm 0.079$                   | $1.175 \pm 0.268$                   | $0.402 \pm 0.071$                   |
| PAT-H (w/DINO-v2)                       | $0.666 \pm 0.074$                   | $1.181 \pm 0.264$                   | $0.397 \pm 0.062$                   |
| PAT-H (w/Kang)                          | <b><math>0.778 \pm 0.010</math></b> | <b><math>1.518 \pm 0.179</math></b> | <b><math>0.339 \pm 0.068</math></b> |

(b) 4X

| Model                                     | $CC_{Attn}$                         | $NSS_{Attn}$                        | $KLD_{Attn}$                        |
|-------------------------------------------|-------------------------------------|-------------------------------------|-------------------------------------|
| Frozen ResNet50+Dec.                      | $0.682 \pm 0.018$                   | $1.510 \pm 0.242$                   | $0.820 \pm 0.249$                   |
| Frozen DINO+Dec.                          | $0.659 \pm 0.027$                   | $1.436 \pm 0.236$                   | $0.860 \pm 0.253$                   |
| ProstAttNet (Chakraborty et al., 2022b)   | $0.571 \pm 0.081$                   | $1.178 \pm 0.055$                   | $1.077 \pm 0.162$                   |
| PathAttFormer (Chakraborty et al., 2022a) | $0.584 \pm 0.079$                   | $1.212 \pm 0.093$                   | $1.074 \pm 0.101$                   |
| PAT-H (w/ DINO)                           | $0.739 \pm 0.029$                   | $1.711 \pm 0.360$                   | $0.473 \pm 0.068$                   |
| PAT-H (w/DINO-v2)                         | $0.738 \pm 0.029$                   | $1.710 \pm 0.362$                   | <b><math>0.473 \pm 0.055</math></b> |
| PAT-H (w/Kang)                            | <b><math>0.765 \pm 0.023</math></b> | <b><math>2.223 \pm 0.360</math></b> | $0.508 \pm 0.130$                   |

(c) 10X

| Model                                   | $CC_{Attn}$                         | $NSS_{Attn}$                        | $KLD_{Attn}$                        |
|-----------------------------------------|-------------------------------------|-------------------------------------|-------------------------------------|
| Frozen ResNet50+Dec.                    | $0.372 \pm 0.042$                   | $1.910 \pm 0.277$                   | $2.361 \pm 0.503$                   |
| Frozen DINO+Dec.                        | $0.365 \pm 0.062$                   | $1.892 \pm 0.271$                   | $2.369 \pm 0.511$                   |
| ProstAttNet (Chakraborty et al., 2022b) | $0.280 \pm 0.066$                   | $1.348 \pm 0.078$                   | $2.287 \pm 0.411$                   |
| PAT-H (w/ DINO)                         | $0.417 \pm 0.065$                   | $2.266 \pm 0.368$                   | $1.741 \pm 0.349$                   |
| PAT-H (w/DINO-v2)                       | $0.419 \pm 0.062$                   | $2.264 \pm 0.377$                   | $1.731 \pm 0.341$                   |
| PAT-H (w/Kang)                          | <b><math>0.438 \pm 0.039</math></b> | <b><math>2.593 \pm 0.315</math></b> | <b><math>1.707 \pm 0.348</math></b> |

(d) 20X

Table 1: Comparison of 5-fold cross-validation performance from our models (red) and the baseline models (blue) for 25 test H&E WSIs of prostate cancer at different magnifications. PathAttFormer (Chakraborty et al., 2022a) is evaluated only at 10X, per their original implementation.

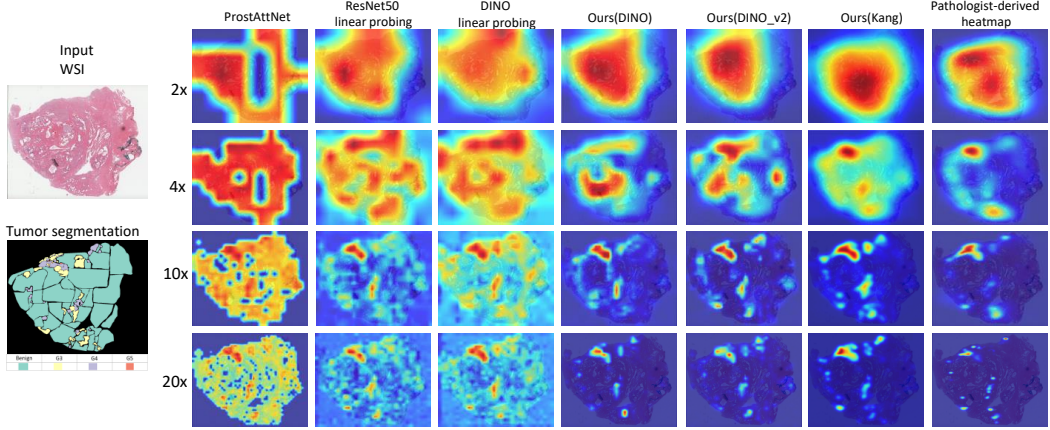

Figure 1: Comparison of attention heatmap prediction performance from our PAT-H model compared to three baselines (left three columns) and the attention ground truth from pathologists. Our PAT-H model better predicts the ground-truth heatmaps compared to the other baselines across all magnifications.

| Model                        | $CC_{Seg}$   | $NSS_{Seg}$  | $KLD_{Seg}$  |
|------------------------------|--------------|--------------|--------------|
| PAT-Heatmap - Specialist     | 0.285        | 1.032        | 2.487        |
| PAT-Heatmap - Non-Specialist | <b>0.314</b> | <b>1.027</b> | <b>2.418</b> |

(a) 2X

| Model                        | $CC_{Seg}$   | $NSS_{Seg}$  | $KLD_{Seg}$  |
|------------------------------|--------------|--------------|--------------|
| PAT-Heatmap - Specialist     | <b>0.406</b> | <b>1.263</b> | <b>2.186</b> |
| PAT-Heatmap - Non-Specialist | 0.386        | 1.253        | 2.250        |

(b) 4X

| Model                        | $CC_{Seg}$   | $NSS_{Seg}$  | $KLD_{Seg}$  |
|------------------------------|--------------|--------------|--------------|
| PAT-Heatmap - Specialist     | <b>0.582</b> | <b>1.851</b> | <b>1.584</b> |
| PAT-Heatmap - Non-Specialist | 0.561        | 1.814        | 1.690        |

(c) 10X

| Model                        | $CC_{Seg}$   | $NSS_{Seg}$  | $KLD_{Seg}$  |
|------------------------------|--------------|--------------|--------------|
| PAT-Heatmap - Specialist     | <b>0.592</b> | <b>2.619</b> | <b>1.382</b> |
| PAT-Heatmap - Non-Specialist | 0.566        | 2.310        | 1.563        |

(d) 20X

Table 2: Performance comparison between our attention heatmap prediction model (using DINO features) trained on specialist data and the same model trained on non-specialist (general pathologists and residents) attention data, based on the spatial overlap between the predicted heatmap and the binary tumor segmentation map, on 17 test H&E WSIs of prostate cancer at different magnifications.

| Method               | Token Similarity (TokSimScan) $\uparrow$ |             |             |             |             |             | NSS $\uparrow$ | AUC $\uparrow$ |
|----------------------|------------------------------------------|-------------|-------------|-------------|-------------|-------------|----------------|----------------|
|                      | Overall                                  | 1X          | 2X          | 4X          | 10X         | 20X         |                |                |
| PAT-ProbMag (2X+4X)  | 0.75                                     | 0.79        | 0.79        | 0.81        | 0.70        | 0.65        | 0.76           | 0.70           |
| PAT-ProbMag (2X+20X) | 0.79                                     | <b>0.82</b> | <b>0.81</b> | 0.79        | 0.69        | <b>0.84</b> | 0.87           | 0.72           |
| PAT-ProbMag (2X+10X) | <b>0.80</b>                              | 0.78        | 0.80        | <b>0.83</b> | <b>0.77</b> | 0.81        | <b>0.99</b>    | <b>0.74</b>    |

Table 3: Comparison of the prediction performance (averaged over the 5 folds) using 4X, 10X, and 20X feature (Kang) encodings from our PAT-H sub-network for constructing the high-resolution feature space of our scanpath prediction sub-network. Using 10X feature encodings for high resolution feature space produces the best results.

| Method                        | Token Similarity (TokSimScan) $\uparrow$ |             |             |             |             |             | NSS $\uparrow$ | AUC $\uparrow$ |
|-------------------------------|------------------------------------------|-------------|-------------|-------------|-------------|-------------|----------------|----------------|
|                               | Overall                                  | 1X          | 2X          | 4X          | 10X         | 20X         |                |                |
| PAT-ProbMag (w/ DINO-Vanilla) | 0.59                                     | <b>0.79</b> | 0.78        | 0.61        | 0.45        | 0.56        | -0.39          | 0.40           |
| PAT-ProbMag (w/ Kang-Vanilla) | 0.71                                     | 0.70        | 0.73        | 0.73        | 0.69        | 0.68        | 0.97           | <b>0.75</b>    |
| PAT-ProbMag (w/ DINO-PAT-H)   | 0.73                                     | 0.71        | 0.76        | 0.76        | 0.72        | 0.72        | 0.83           | 0.71           |
| PAT-ProbMag (w/ Kang-PAT-H)   | <b>0.80</b>                              | 0.78        | <b>0.80</b> | <b>0.83</b> | <b>0.77</b> | <b>0.81</b> | <b>0.99</b>    | 0.74           |

Table 4: Comparison of the performance of our PAT model using DINO encodings (pre-trained on ImageNet) with feature encodings from our PAT-H sub-network, for the scanpath prediction task (averaged over the 5 folds). Our PAT-H encodings based on the model trained using the *Kang* features produce the best results.

#### 4. Ablation studies: scanpath prediction

**Effect of fixation number on attention consistency.** Figure 2 illustrates that the joint spatial variance in fixation locations ( $X + Y$ ) on a WSI (averaged over all WSIs in our training dataset) increases with fixation number, particularly beyond 60 fixations. This implies that while early fixations tend to be more concentrated and task-driven, likely focusing on diagnostically relevant regions, longer scanpaths (beyond 60 fixations) show higher spatial dispersion, indicating that these later fixations are more exploratory. As shown in the plot, fixation variance continues to grow, while the number of scanpaths contributing to each bin drops sharply beyond 60. This means fewer consistent behavioral patterns exist in this range, and the data is less reliable for modeling or evaluation. Given this, evaluating very long scanpaths could introduce noise, reduce comparability across subjects, and misrepresent model performance by focusing on less consistent parts of the viewing behavior. Limiting evaluation to scanpaths of length  $N \leq 60$  ensures that comparisons are based on the more consistent and clinically meaningful

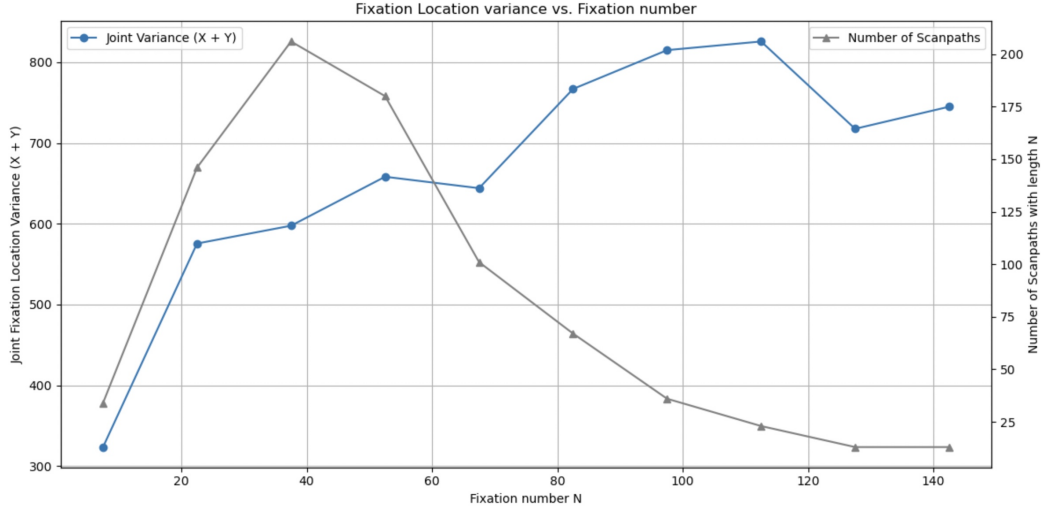

Figure 2: Spatial variance of the fixation locations (x,y) vs. fixation number. The plot shows that the variance of the fixation locations increases with increasing fixation number.

portions of attention.

**Feature resolution.** We ablated our model by using multi-resolutional feature encodings from different magnification levels. In Table 3, we compare the prediction performance of our model using 4X, 10X, and 20X feature encodings for the high-resolution information and found that 10X feature encodings produce the best results. This shows that 10X, because it is the most frequently used magnification level, produces the best feature space for predicting scanpaths.

**Feature Encodings.** We evaluated the predictive performance of our model using various types of feature encodings. In Table 4, we compare the scan-path prediction performance using pre-trained self-supervised DINO encodings (trained on ImageNet-1k (Deng et al., 2009)) to the feature encodings generated by our *PAT-H* sub-network. While DINO-v2 encodings could also have been considered, our experiments in Table 1 indicated slightly better performance using DINO embeddings, so we proceeded with DINO. The results show that feature encodings derived from our *PAT-H* sub-network lead to improved performance across all metrics. This ablation highlights the superior effectiveness of our model’s feature encodings in capturing pathologist attention compared to pre-trained DINO features.

| Method                   | Token Similarity (TokSimScan) $\uparrow$ |                                   |                                   |                                   |                                   |                                   | NSS $\uparrow$                    | AUC $\uparrow$                    |
|--------------------------|------------------------------------------|-----------------------------------|-----------------------------------|-----------------------------------|-----------------------------------|-----------------------------------|-----------------------------------|-----------------------------------|
|                          | Overall                                  | 1X                                | 2X                                | 4X                                | 10X                               | 20X                               |                                   |                                   |
| PAT-DetMag (DINO-PAT-H)  | 0.15 $\pm$ 0.14                          | <b>0.91 <math>\pm</math> 0.06</b> | 0.00 $\pm$ 0.00                   | 0.00 $\pm$ 0.00                   | 0.00 $\pm$ 0.00                   | 0.22 $\pm$ 0.53                   | 0.78 $\pm$ 0.18                   | 0.70 $\pm$ 0.15                   |
| PAT-ProbMag (DINO-PAT-H) | <b>0.73 <math>\pm</math> 0.04</b>        | 0.71 $\pm$ 0.06                   | <b>0.76 <math>\pm</math> 0.08</b> | <b>0.76 <math>\pm</math> 0.04</b> | <b>0.72 <math>\pm</math> 0.04</b> | <b>0.72 <math>\pm</math> 0.04</b> | <b>0.83 <math>\pm</math> 0.13</b> | <b>0.71 <math>\pm</math> 0.04</b> |

Table 5: Quantitative evaluation of the prediction performance of our PAT deterministic (PAT-DetMag) and probabilistic (PAT-ProbMag) models (using DINO features) with 5-fold cross-validation. Our PAT-ProbMag model outperforms the PAT-DetMag version.

| Method                        | Token Similarity (TokSimScan) $\uparrow$ |                                   |                                   |                                   |                                   |                                   | NSS $\uparrow$                    | AUC $\uparrow$                    |
|-------------------------------|------------------------------------------|-----------------------------------|-----------------------------------|-----------------------------------|-----------------------------------|-----------------------------------|-----------------------------------|-----------------------------------|
|                               | Overall                                  | 1X                                | 2X                                | 4X                                | 10X                               | 20X                               |                                   |                                   |
| PAT-ProbMag-3way (DINO-PAT-H) | 0.71 $\pm$ 0.07                          | <b>0.72 <math>\pm</math> 0.04</b> | 0.74 $\pm$ 0.06                   | 0.74 $\pm$ 0.07                   | 0.71 $\pm$ 0.05                   | 0.71 $\pm$ 0.09                   | 0.81 $\pm$ 0.17                   | 0.71 $\pm$ 0.06                   |
| PAT-ProbMag-6way (DINO-PAT-H) | <b>0.73 <math>\pm</math> 0.04</b>        | 0.71 $\pm$ 0.06                   | <b>0.76 <math>\pm</math> 0.08</b> | <b>0.76 <math>\pm</math> 0.04</b> | <b>0.72 <math>\pm</math> 0.04</b> | <b>0.72 <math>\pm</math> 0.04</b> | <b>0.83 <math>\pm</math> 0.13</b> | <b>0.71 <math>\pm</math> 0.04</b> |

Table 6: Quantitative comparison of the prediction performance of two versions (3-way vs. 6-way magnification prediction) of our probabilistic PAT-ProbMag model using 5-fold cross-validation. Our PAT-ProbMag model with 6-way magnification classification outperforms the alternative 3-way classification model version by a small margin.

**Probabilistic vs. deterministic magnification prediction.** In the main paper, we primarily considered a probabilistic approach for modeling magnification transitions. To explore the effect of deterministic magnification selection, we additionally evaluated the ‘‘PAT-DetMag’’ variant, where the magnification level for the next viewport fixation is deterministically selected using the *argmax* operator over the prediction logits.

As shown in Table 5, deterministic magnification prediction leads to substantially worse performance across all metrics compared to the probabilistic version (PAT-ProbMag). This highlights the importance of probabilistic modeling in capturing the inherent variability and uncertainty in pathologist magnification behavior during WSI reading.

**Magnification Prediction: 3-way vs. 6-way prediction performance.** In Table 6, we compare two versions of our PAT-ProbMag model: (1) a 6-way magnification prediction model that outputs logits over all magnification levels (1X–40X), followed by probabilistic sampling of  $\Delta m \in \{-1, 0, 1\}$  based on the current magnification level; and (2) an alternative 3-way model that directly predicts  $\Delta m$  as a directional change, adding the predicted shift to the current magnification level. We find that the 6-way model outperforms the 3-way variant. This improvement likely stems from the richer contextual representations learned through the more granular 6-way classification.

## References

- Bylinskii, Z., Judd, T., Oliva, A., Torralba, A., Durand, F., 2018. What do different evaluation metrics tell us about saliency models? *IEEE transactions on pattern analysis and machine intelligence* 41, 740–757.
- Caron, M., Touvron, H., Misra, I., Jégou, H., Mairal, J., Bojanowski, P., Joulin, A., 2021. Emerging properties in self-supervised vision transformers, in: *Proceedings of the IEEE/CVF international conference on computer vision*, pp. 9650–9660.
- Chakraborty, S., Gupta, R., Ma, K., Govind, D., Sarder, P., Choi, W.T., Mahmud, W., Yee, E., Allard, F., Knudsen, B., et al., 2022a. Predicting the visual attention of pathologists evaluating whole slide images of cancer, in: *International Workshop on Medical Optical Imaging and Virtual Microscopy Image Analysis*, Springer. pp. 11–21.
- Chakraborty, S., Ma, K., Gupta, R., Knudsen, B., Zelinsky, G.J., Saltz, J.H., Samaras, D., 2022b. Visual attention analysis of pathologists examining whole slide images of prostate cancer, in: *2022 IEEE 19th International symposium on biomedical imaging (ISBI)*, IEEE. pp. 1–5.
- Deng, J., Dong, W., Socher, R., Li, L.J., Li, K., Fei-Fei, L., 2009. Imagenet: A large-scale hierarchical image database, in: *2009 IEEE Conference on Computer Vision and Pattern Recognition (CVPR)*, IEEE. pp. 248–255. doi:10.1109/CVPR.2009.5206848.
- Kang, M., Song, H., Park, S., Yoo, D., Pereira, S., 2023. Benchmarking self-supervised learning on diverse pathology datasets, in: *Proceedings of the IEEE/CVF Conference on Computer Vision and Pattern Recognition*, pp. 3344–3354.
- Oquab, M., Darcet, T., Moutakanni, T., Vo, H.V., Szafraniec, M., Khalidov, V., Fernandez, P., Haziza, D., Massa, F., El-Nouby, A., Howes, R., Huang, P.Y., Xu, H., Sharma, V., Li, S.W., Galuba, W., Rabbat, M., Assran, M., Ballas, N., Synnaeve, G., Misra, I., Jegou, H., Mairal, J., Labatut, P., Joulin, A., Bojanowski, P., 2023. DINOv2: Learning robust visual features without supervision.
- Yang, Z., Mondal, S., Ahn, S., Xue, R., Zelinsky, G., Hoai, M., Samaras, D., 2024. Unifying top-down and bottom-up scanpath prediction using

transformers, in: Proceedings of the IEEE/CVF Conference on Computer Vision and Pattern Recognition, pp. 1683–1693.
